# Supplementary material for: Large Language Models Are Active Critics in NLG Evaluation
Source: arXiv:2410.10724 source file (2025-02-17)
Supplement: Supplementary file 1 [file 07_Effectiveness_Multi_stage_Appendix.tex]

\begin{table}[htp]
\centering
\resizebox{0.95\textwidth}{!}{
\begin{tabular}{lcccccccc}
\toprule
~ & \multicolumn{4}{c}{before optimization} & \multicolumn{4}{c}{after optimization} \\
\cmidrule(lr){2-5} \cmidrule(lr){6-9}  ~& SummEval & TopicalChat & SFRES &OpenMEVA & SummEval & TopicalChat & SFRES &OpenMEVA \\
\midrule

\textbf{Ours} & \textbf{0.5702} &\textbf{0.6286} &\textbf{0.3637} &\textbf{0.4774}&\textbf{0.6354} &\underline{0.6286}& \textbf{0.3564}& \textbf{0.5484}\\

\midrule
- stage1 & 0.5349 &0.5078&0.2757&0.4049& 0.5928& 0.5164& 0.2761& 0.4131\\

- stage2 &  0.5686 &0.56&0.3369&0.3772&0.5854& 0.5826& 0.3406& 0.4098\\

- stage3 & 0.5277 &0.5708 &0.344 &\underline{0.4629}&0.5479& \textbf{0.646}& 0.413&0.5235\\

- stage4 & \underline{0.5897} &\underline{0.579}&\underline{0.3501}&0.4623&\underline{0.6204} & 0.5903& \underline{0.3467}& \underline{0.533}\\

\bottomrule
\end{tabular}
}
\caption{Effectiveness of multi-stage. We report Pearson ($\gamma$) correlations in four scenarios where stages1 to stage4 are individually removed. }
\label{tab:multi-stage_Pearson}
\end{table}

\begin{table}[htp]
\centering
\resizebox{0.95\textwidth}{!}{
\begin{tabular}{lcccccccc}
\toprule
~ & \multicolumn{4}{c}{before optimization} & \multicolumn{4}{c}{after optimization} \\
\cmidrule(lr){2-5} \cmidrule(lr){6-9}  ~& SummEval & TopicalChat & SFRES &OpenMEVA & SummEval & TopicalChat & SFRES &OpenMEVA \\
\midrule

\textbf{Ours} &\underline{ 0.504}& \textbf{0.6402}&\textbf{0.3171}& \textbf{0.4668}&\textbf{0.5507}&\underline{0.6402}& \underline{0.3166}& \textbf{0.5325}\\

\midrule
- stage1 & 0.454& 0.5010& 0.2274& 0.3807&0.4766& 0.5290& 0.2386& 0.4103\\

- stage2 &  \textbf{0.5111}& 0.5367&0.2852& 0.368&\underline{0.5306}& 0.5577& 0.3092& 0.3909\\

- stage3 & 0.5002& \underline{0.5886}& 0.2809& 0.46& 0.5205& \textbf{0.6529}&\textbf{0.3298}& 0.5217\\

- stage4 & 0.4953& 0.5563& \underline{0.3021}& \underline{0.4611}&0.5219& 0.5881& 0.3059& \underline{0.5224}\\

\bottomrule
\end{tabular}
}
\caption{Effectiveness of multi-stage. We report Spearman ($\rho$) correlations in four scenarios where stages1 to stage4 are individually removed. }
\label{tab:multi-stage_Spearman}
\end{table}
